# Supplementary material for: To Compress or Not to Compress- Self-Supervised Learning and Information Theory: A Review
Source: arXiv:2304.09355 source file (2023-11-21)
Supplement: Supplementary file 1 [file 10_appendices.tex]

\begin{appendices}

\crefalias{section}{appsec}
\crefalias{subsection}{appsec}
\crefalias{subsubsection}{appsec}

\setcounter{equation}{0}

\onecolumn

%%%%%%%%%%%%%%%%%%%%%%%%%%%

\section*{\LARGE Supplementary Material}
\label{sec:appendix}

\section{Lower bounds on $\EE_{x^\prime}\left[\log q(z|x^\prime)\right]$}
\label{app:33}

In this section of the supplementary material, we present the full derivation of the lower bound on $ \EE_{x^\prime}\left[\log q(z|x^\prime)\right]$.
Because $Z^\prime|X^\prime$ is a Gaussian, we can write it as $Z^\prime = \mu(x^\prime) + L(x^\prime)\epsilon$ where  $\epsilon \sim \mathcal{N}(0, 1) $ and  $L(x^\prime)^TL(x^\prime) = \Sigma(x^\prime)$. Now, setting $\Sigma_r = I$, will give us:
 \begin{align}
 \label{eq:logzz_e}
 \begin{split}
    &
     \EE_{x^\prime}\left[\log q(z|x^\prime)\right]  
     \\
     \geq &  
     \EE_{z^\prime|x^\prime}\left[\log q(z|z^\prime)\right]
      \end{split}
     \\=&
     \EE_{z^\prime|x^\prime}\left[\frac{d}{2}\log 2\pi - \frac12 \left(z-z^\prime\right)^T\left(I)\right)^{-1}\left(z-z^\prime\right)\right] \\ = &
     \frac{d}{2}\log 2\pi - \frac12 \EE_{z^\prime \mid x^\prime, }\left[\left(z-z^\prime\right)^2\right] \\ = &
      \frac{d}{2}\log 2\pi - \frac12 \EE_{ \epsilon}\left[\left(z-\mu(x^\prime) - L(x^\prime)\epsilon\right)^2\right] \\ =
      &
       \frac{d}{2}\log 2\pi - \frac12 \EE_{ \epsilon}\left[\left(z-\mu(x^\prime)\right)^2 - 2\left(z - \mu(x^\prime)*L(x^\prime) \epsilon\right) +\left(\left(L(x^\prime)\epsilon\right)^T\left(L(x^\prime) \epsilon\right)\right)\right] \\ = &
       \frac{d}{2}\log 2\pi - \frac12 \EE_{\epsilon}\left[\left(z-\mu(x^\prime)\right)^2\right] +
       \left(z-\mu(x^\prime)L(x^\prime)\right)\EE_{\epsilon}\left[\epsilon\right]-\frac{1}{2}\EE_{\epsilon}\left[\epsilon^T L(x^\prime)^T L(x^\prime) \epsilon\right] \\ = &
      \frac{d}{2}\log 2\pi - \frac12 \left(z-\mu(x^\prime)\right)^2 -\frac{1}{2}Tr\log\Sigma(x^\prime)
 \end{align}
 where $\EE_{x^\prime}\left[\log q(z|x^\prime)\right] =  \EE_{x^\prime}\left[\log \EE_{z^\prime|x^\prime} \left[q(z|z^\prime)\right]\right] \geq \EE_{z^\prime}\left[\log q(z|z^\prime)\right]  $ by   Jensen's inequality, $\EE_{\epsilon}[\epsilon]=0$  and 
 $\EE_{\epsilon}\left[\epsilon\left(L(x^\prime)^T L(x^\prime \right)\epsilon\right] = Tr\log\Sigma(x^\prime)$ by the Hutchinson's estimator.
 \begin{align}
     \EE_{z|x}\left[\EE_{z^\prime|x^\prime}\left[\log q(z|z^\prime)\right]\right] = &
     \EE_{z|x}\left[\frac{d}{2}\log 2\pi - \frac12 \left(z-\mu(x^\prime)\right)^2 -\frac{1}{2}Tr \log \Sigma(x^\prime)\right] \\ =&
          \frac{d}{2}\log 2\pi - \frac12 \EE_{z|x}\left[ \left(z-\mu(x^\prime)\right)^2\right] -\frac{1}{2}Tr \log \Sigma(x^\prime) \\ = &
              \frac{d}{2}\log 2\pi - \frac12 \EE_{\epsilon}\left[ \left(\mu(x) +L(x)\epsilon-\mu(x^\prime)\right)^2\right] -\frac{1}{2}Tr \log \Sigma(x^\prime) \\
              \begin{split}
              = &
                \frac{d}{2}\log 2\pi -  \frac12 \EE_{\epsilon}\left[ \left(\mu(x) -\mu(x^\prime)\right)^2\right] +\EE_{\epsilon}\left[\left(\mu(x) - \mu(x^\prime)\right)L(x)\epsilon\right] \\&-\frac 12\EE_{\epsilon}\left[\epsilon^TL(x)^TL(x)\epsilon\right] -\frac{1}{2}Tr\log \Sigma(x^\prime)
                \end{split}
                \\ = &
                    \frac{d}{2}\log 2\pi -  \frac12  \left(\mu(x) -\mu(x^\prime)\right)^2 -\frac 12Tr\log\Sigma(x) -\frac{1}{2}Tr\log\Sigma(x^\prime)
                    \\ =&
                        \frac{d}{2}\log 2\pi -  \frac12  \left(\mu(x) -\mu(x^\prime)\right)^2 -\frac 12 \log \left( |\Sigma(x)|  \cdot |\Sigma(x^\prime)|\right)
 \end{align}

\clearpage

\section{Data Distribution after Deep Network Transformation}
\label{app:2}

\begin{thm}
Given the setting of \cref{eq:x_density} the unconditional DNN output density denoted as $Z$ approximates (given the truncation of the Gaussian on its effective support that is included within a single region $\omega$ of the DN's input space partition) a mixture of the affinely transformed distributions $\bx|\bx^*_{n(\bx)}$ e.g. for the Gaussian case
$$Z\hspace{-0.1cm} \sim\hspace{-0.1cm} \sum_{n=1}^{N}\mathcal{N}\hspace{-0.1cm}\left(\hspace{-0.1cm}\bA_{\omega(\bx^*_{n})}\bx^*_{n}+\bb_{\omega(\bx^*_{n})},\bA^T_{\omega(\bx^*_{n})}\Sigma_{\bx^*_{n}}\bA_{\omega(\bx^*_{n})}\hspace{-0.1cm}\right)^{T=n},$$
where $\omega(\bx^*_{n})=\omega \in \Omega \iff \bx^*_{n} \in \omega$ is the partition region in which the prototype $\bx^*_{n}$ lives in.
\end{thm}
%\vspace{-0.2cm}
% \vspace{3pt}
\begin{proof}
 We know that If $\int_{\omega}p(\bx|\bx^*_{n(\bx)})d\bx \approx 1$ then $f$ is linear within the effective support of $p$. Therefore, any sample from $p$ will almost surely lie within a single region $\omega \in \Omega$ and therefore the entire mapping can be considered linear with respect to $p$. Thus, the output distribution is a linear transformation of the input distribution based on the per-region affine mapping.
\end{proof}

% \clearpage

\section{Generalization Bound}

The following theorem is the complete version of Theorem \ref{thm:1}: 

\begin{thm} \label{thm:11}
For any $\delta>0$, with probability at least $1-\delta$, the following holds: \begin{align}
\EE_{x,y}[\ell_{x,y}(w_{S})]\le c I_{\bS}(f_\theta) +\frac{2}{\sqrt{m}}\|\Pb_\hZ Y_\bS\|_{F}+\frac{1}{\sqrt{n}}  \|\Pb_\tZ Y_{S}\|_F +Q_{m,n},
\end{align}
where
\begin{align*}
Q_{m,n} &=  c \left(\frac{2\tilde \Rcal_{m}(\Fcal)}{\sqrt{m}}+\tau \sqrt{\frac{\ln(3/\delta)}{2m}}+\tau_{\bS} \sqrt{\frac{\ln(3/\delta)}{2n}}\right)
\\ & \quad +\kappa_{S}   \sqrt{\frac{2\ln(6|\Ycal|/\delta)}{2n}}  \sum_{y\in \Ycal} \left(\sqrt{\hp(y)}+\sqrt{p(y)}\right)
 \\ & \quad + \frac{4\Rcal_{m}(\Wcal \circ \Fcal)}{\sqrt{m}}+2\kappa \sqrt{\frac{\ln(4/\delta)}{2m}} + 2\kappa_{\bS} \sqrt{\frac{\ln(4/\delta)}{2n} }. 
\end{align*}
\end{thm}
\begin{proof}
The complete proof is presented in Appendix \ref{app:1:1}.
\end{proof}

The bound in the complete version of Theorem \ref{thm:11} is   better than the one in the informal version of Theorem \ref{thm:1}, because of the factor $c$. The factor $c$ measures the difference between the minimum norm solution  $W_S$ of the labeled training data and the minimum norm solution $W_\bS$ of the unlabeled training data. Thus, the factor $c$ also decreases towards zero as $n$ and $m$ increase. Moreover, if the labeled and unlabeled training data are similar, the value of $c$ is small, decreasing the generalization bound further, which makes sense. Thus, we can view the factor $c$ as a measure on the distance between the labeled training data and the unlabeled training data. 

We obtain the informal version from the complete version of Theorem \ref{thm:1} by the following reasoning to simplify the notation in the main text. We have that $ c I_{\bS}(f_\theta) +c\frac{2\tilde \Rcal_{m}(\Fcal)}{\sqrt{m}}= I_{\bS}(f_\theta) +\frac{2\tilde \Rcal_{m}(\Fcal)}{\sqrt{m}}+Q$, where $Q=(c-1)( I_{\bS}(f_\theta)+\frac{2\tilde \Rcal_{m}(\Fcal)}{\sqrt{m}}) \le \varsigma \rightarrow 0$ as as $m,n \rightarrow \infty$, since $c \rightarrow 0$ as $m,n \rightarrow \infty$. However, this reasoning is used only to simplify the notation in the main text. The bound in the complete version of Theorem \ref{thm:1} is more accurate and indeed tighter  than the one in the informal version.

In Theorem \ref{thm:1}, $Q_{m,n} \rightarrow 0$ as $m,n\rightarrow \infty$ if $\frac{\tilde \Rcal_{m}(\Fcal)}{\sqrt{m}} \rightarrow 0$ as $m\rightarrow \infty$.
Indeed, this typically holds because  $\tilde \Rcal_{m}(\Fcal)=O(1)$ as $m\rightarrow \infty$ for  typical choices of $\Fcal$, including deep  neural networks \citep{bartlett2017spectrally,kawaguchi2018generalization,golowich2018size} as well as other common machine learning models \citep{bartlett2002rademacher,mohri2012foundations,shalev2014understanding, shwartz-ziv2023what}.

\subsection{Proof of Theorem \ref{thm:1}} \label{app:1:1}
\begin{proof}[Proof of Theorem \ref{thm:1}]
Let $W=W _{S}$ where $W_S$ is the the minimum norm solution as  $W_S =\mini_{W'} \|W'\|_{F}$ s.t. $W'\in \argmin_{W} \frac{1}{n} \sum_{i=1}^n \|W f_\theta(x_i)-y_i\|^2$. Let $W^*=W_\bS$ where $W_\bS$ is the minimum norm solution as $W^{*}=W_{\bS}=\mini_{W'} \|W'\|_{F}$ s.t. $W'\in \argmin_{W} \frac{1}{m} \sum_{i=1}^{m} \|W f_\theta(\xp_{i})-g^*(\xp_i)\|^2$.  Since $y=g^{*}(x)$, 
\begin{align*}
y=g^{*}(x)  \pm W^*  f_\theta(x) =W^*  f_\theta(x) +(g^{*}(x)-W^*  f_\theta(x))=W^*  f_\theta(x) +\varphi(x) \end{align*}
where $\varphi(x)=g^{*}(x)-W^*  f_\theta(x)$.
Define $L_{S}(w)= \frac{1}{n} \sum_{i=1}^n \|W f_\theta(x_i)-y_i\|$. Using these, \begin{align*}
L_{S}(w) &= \frac{1}{n} \sum_{i=1}^n \|W f_\theta(x_i)-y_i\|
\\ & =\frac{1}{n} \sum_{i=1}^n \|W f_\theta(x_i)-W^*  f_\theta(x_{i}) -\varphi(x_{i})\| \\ & \ge\frac{1}{n} \sum_{i=1}^n \|W f_\theta(x_i)-W^*  f_\theta(x_{i})\| -\frac{1}{n} \sum_{i=1}^n\|\varphi(x_{i})\| 
\\ & =\frac{1}{n} \sum_{i=1}^n \|\tW f_\theta(x_i)\| - \frac{1}{n} \sum_{i=1}^n \|\varphi(x_{i})\| 
\end{align*}
where $\tW =W-W^*$. We now consider new fresh samples $\bbx_{i} \sim\Dcal _{y_{i}}$ for $i=1,\dots, n$ to rewrite the above further as:
\begin{align*}
L_{S}(w) &\ge \frac{1}{n} \sum_{i=1}^n \|\tW f_\theta(x_i)\pm\tW f_\theta(\bbx_i)\| - \frac{1}{n} \sum_{i=1}^n \|\varphi(x_{i})\|
\\ & =\frac{1}{n} \sum_{i=1}^n \|\tW f_\theta(\bbx_i)-(\tW f_\theta(\bbx_i)-\tW f_\theta(x_i))\| - \frac{1}{n} \sum_{i=1}^n \|\varphi(x_{i})\| 
\\ & \ge\frac{1}{n} \sum_{i=1}^n \|\tW f_\theta(\bbx_i)\| -\frac{1}{n} \sum_{i=1}^{n}\|\tW f_\theta(\bbx_i)-\tW f_\theta(x_i)\| - \frac{1}{n} \sum_{i=1}^n \|\varphi(x_{i})\| \\ & =\frac{1}{n} \sum_{i=1}^n \|\tW f_\theta(\bbx_i)\| -\frac{1}{n} \sum_{i=1}^{n}\|\tW (f_\theta(\bbx_i)-f_\theta(x_i))\| - \frac{1}{n} \sum_{i=1}^n \|\varphi(x_{i})\| \end{align*}   
This implies that 
$$
\frac{1}{n} \sum_{i=1}^n \|\tW f_\theta(\bbx_i)\| \le L_{S}(w)+\frac{1}{n} \sum_{i=1}^{n}\|\tW (f_\theta(\bbx_i)-f_\theta(x_i))\| + \frac{1}{n} \sum_{i=1}^n \|\varphi(x_{i})\|.
$$
Furthermore, since $y=W^*  f_\theta(x) +\varphi(x)$, by writing $\bby_{i}=W^*  f_\theta(\bbx_i) +\varphi(\bbx_i)$ (where $\bby_i = y_i$ since  $\bbx_{i} \sim\Dcal _{y_{i}}$ for $i=1,\dots, n$),
\begin{align*}
\frac{1}{n} \sum_{i=1}^n \|\tW f_\theta(\bbx_i)\| &=\frac{1}{n} \sum_{i=1}^n \|Wf_\theta(\bbx_i)-W^* f_\theta(\bbx_i)\|
\\ & =\frac{1}{n} \sum_{i=1}^n \|Wf_\theta(\bbx_i)-\bby_i+\varphi(\bbx_i)\| \\ & \ge\frac{1}{n} \sum_{i=1}^n \|Wf_\theta(\bbx_i)-\bby_i\|-\frac{1}{n} \sum_{i=1}^n\|\varphi(\bbx_i) \|  
\end{align*}
Combining these, we have that 
\begin{align} \label{eq:1}
\frac{1}{n} \sum_{i=1}^n \|Wf_\theta(\bbx_i)-\bby_i\| &\le  L_{S}(w)+\frac{1}{n} \sum_{i=1}^{n}\|\tW (f_\theta(\bbx_i)-f_\theta(x_i))\| 
\\ \nonumber & \quad + \frac{1}{n} \sum_{i=1}^n \|\varphi(x_{i})\|+\frac{1}{n} \sum_{i=1}^n\|\varphi(\bbx_i) \|. 
\end{align}
 To bound the left-hand side of \eqref{eq:1}, we now analyze the following random variable:
\begin{align} \label{eq:5}
\EE_{X,Y}[\|W _{S}f_\theta(X)-Y\|]   - \frac{1}{n} \sum_{i=1}^n \|W_{S}f_\theta(\bbx_i)-\bby_i\|,
\end{align}
where $\bby_i = y_i$ since  $\bbx_{i} \sim\Dcal _{y_{i}}$ for $i=1,\dots, n$. Importantly, this means that  as $W_{S}$ depends on $y_i$, $W_{S}$ depends on $\bby_i$. Thus, the collection of random variables $\|W_{S}f_\theta(\bbx_1)-\bby_1\|,\dots,\|W_{S}f_\theta(n_n)-\bby_n\|$ is \textit{not} independent. Accordingly, we cannot apply standard concentration inequality to bound  \eqref{eq:5}.
A standard approach in learning theory is to first bound   \eqref{eq:5} by $\EE_{x,y}\|W _{S}f_\theta(x)-y\|   - \frac{1}{n} \sum_{i=1}^n \|W_{S}f_\theta(\bbx_i)-\bby_i\| \le\sup_{W \in \Wcal}\EE_{x,y}\|Wf_\theta(x)-y\|   - \frac{1}{n} \sum_{i=1}^n \|Wf_\theta(\bbx_i)-\bby_i\|$ for some hypothesis space $\Wcal$ (that is independent of $S$) and realize that the right-hand side now contains the collection of independent random variables $\|W_{}f_\theta(\bbx_1)-\bby_1\|,\dots,\|W_{}f_\theta(n_n)-\bby_n\|$ , for which we can utilize  standard concentration inequalities. This reasoning leads to the Rademacher complexity of  the hypothesis space $\Wcal$. However, the complexity of the hypothesis space $\Wcal$ can be very large, resulting into a loose bound.  In this proof, we show that we can avoid the dependency on hypothesis space $\Wcal$ by using a very different approach with conditional expectations to take care the dependent random variables $\|W_{S}f_\theta(\bbx_1)-\bby_1\|,\dots,\|W_{S}f_\theta(n_n)-\bby_n\|$.
Intuitively, we utilize the fact that for these dependent random variables, there are a structure of  conditional independence, conditioned on each $y \in \Ycal$.  

We first write the expected loss as the sum of the conditional expected loss:
\begin{align*}
\EE_{X,Y}[\|W _{S}f_\theta(X)-Y\|]&=\sum_{y\in \Ycal} \EE_{X,Y}[\|W _{S}f_\theta(X)-Y\| \mid Y = y]\Pr(Y =  y)
\\ & =\sum_{y\in \Ycal}\EE_{X_{y}}[\|W _{S}f_\theta(X_{y})-y \|]\Pr(Y =  y),
\end{align*}
where $X_{y}$ is the random variable for the conditional with $Y=y$. 
Using this, we  decompose \eqref{eq:5}  into two terms:
\begin{align} \label{eq:6}
&\EE_{X,Y}[\|W _{S}f_\theta(X)-Y\|]   - \frac{1}{n} \sum_{i=1}^n \|W_{S}f_\theta(\bbx_i)-\bby_i\| 
\\ \nonumber & =  \left(\sum_{y\in \Ycal} \EE_{X_{y}}[\|W _{S}f_\theta(X_{y})-y \|]\frac{|\Ical_{y}|}{n}-  \frac{1}{n} \sum_{i=1}^n \|W_{S}f_\theta(\bbx_i)-\bby_i\|\right) \\ \nonumber & \quad+\sum_{y\in \Ycal} \EE_{X_{y}}[\|W _{S}f_\theta(X_{y})-y \|]\left(\Pr(Y =  y)- \frac{|\Ical_{y}|}{n}\right),
\end{align}
where
$$
\Ical_{y}=\{i\in[n]: y_{i}=y\}.
$$
The first term in the right-hand side  of \eqref{eq:6} is further simplified by using 
$$
  \frac{1}{n} \sum_{i=1}^n \|W_{S}f_\theta(\bbx_i)-\bby_i\|=\frac{1}{n}\sum_{y \in \Ycal}  \sum_{i \in \Ical_{y}}  \|W_{S}f_\theta(\bbx_i)-y\|, 
$$
as 
\begin{align*}
 &\sum_{y\in \Ycal} \EE_{X_{y}}[\|W _{S}f_\theta(X_{y})-y \|]\frac{|\Ical_{y}|}{n}-  \frac{1}{n} \sum_{i=1}^n \|W_{S}f_\theta(\bbx_i)-\bby_i\|
 \\ & =\frac{1}{n}\sum_{y \in \tYcal}  |\Ical_{y}|\left(\EE_{X_{y}}[\|W _{S}f_\theta(X_{y})-y \|]-\frac{1}{|\Ical_{y}|}\sum_{i \in \Ical_{y}}\|W_{S}f_\theta(\bbx_i)-y\| \right),
\end{align*}
where $\tYcal=\{y \in \Ycal : |\Ical_{y}| \neq 0\}$. Substituting these into equation \eqref{eq:6} yields
\begin{align} \label{eq:7} 
&\EE_{X,Y}[\|W _{S}f_\theta(X)-Y\|]   - \frac{1}{n} \sum_{i=1}^n \|W_{S}f_\theta(\bbx_i)-\bby_i\|
\\ \nonumber & = \frac{1}{n}\sum_{y \in  \tYcal}  |\Ical_{y}|\left(\EE_{X_{y}}[\|W _{S}f_\theta(X_{y})-y \|]-\frac{1}{|\Ical_{y}|}\sum_{i \in \Ical_{y}}\|W_{S}f_\theta(\bbx_i)-y\| \right)
\\ \nonumber & \quad + \sum_{y\in \Ycal} \EE_{X_{y}}[\|W _{S}f_\theta(X_{y})-y \|]\left(\Pr(Y =  y)- \frac{|\Ical_{y}|}{n}\right)
\end{align}  
Importantly, while $\|W_{S}f_\theta(\bbx_1)-\bby_1\|,\dots, \|W_{S}f_\theta(\bbx_n)-\bby_n\|$ on  the right-hand side of \eqref{eq:7} are dependent random variables, $\|W_{S}f_\theta(\bbx_1)-y\|,\dots,\|W_{S}f_\theta(\bbx_n)-y\|$ are independent random variables since $W_S$ and $\bbx_i$ are independent and $y$ is fixed here. Thus, by using Hoeffding's inequality (Lemma \ref{lemma:trivial:2}), and taking union bounds over $y \in \tYcal$, we have that with probability at least $1-\delta$,
the following holds for all $y \in \tYcal$:
$$
\EE_{X_{y}}[\|W _{S}f_\theta(X_{y})-y \|]-\frac{1}{|\Ical_{y}|}\sum_{i \in \Ical_{y}}\|W_{S}f_\theta(\bbx_i)-y\| \le \kappa_{S} \sqrt{\frac{\ln(|\tYcal|/\delta)}{2|\Ical_{y}|}}. 
$$
This implies that with probability at least $1-\delta$,
\begin{align*}
&\frac{1}{n}\sum_{y \in \tYcal}  |\Ical_{y}|\left(\EE_{X_{y}}[\|W _{S}f_\theta(X_{y})-y \|]-\frac{1}{|\Ical_{y}|}\sum_{i \in \Ical_{y}}\|W_{S}f_\theta(\bbx_i)-y\| \right) 
\\ & \le\frac{\kappa_{S}}{n}\sum_{y \in \tYcal}  |\Ical_{y}| \sqrt{\frac{\ln(|\tYcal|/\delta)}{2|\Ical_{y}|}}
\\ &=\kappa_{S} \left(\sum_{y \in \tYcal} \sqrt{\frac{|\Ical_{y}|}{n}}\right)   \sqrt{\frac{\ln(|\tYcal|/\delta)}{2n}}. 
\end{align*}
Substituting this bound into \eqref{eq:7}, we have that with probability at least $1-\delta$,
\begin{align} \label{eq:8} 
&\EE_{X,Y}[\|W _{S}f_\theta(X)-Y\|]   - \frac{1}{n} \sum_{i=1}^n \|W_{S}f_\theta(\bbx_i)-\bby_i\|
\\ \nonumber & \le \kappa_{S} \left(\sum_{y \in \tYcal} \sqrt{\hp(y)}\right)   \sqrt{\frac{\ln(|\tYcal|/\delta)}{2n}} 
  + \sum_{y\in \Ycal} \EE_{X_{y}}[\|W _{S}f_\theta(X_{y})-y \|]\left(\Pr(Y =  y)- \frac{|\Ical_{y}|}{n}\right)
\end{align} 
where 
$$
\hp(y)= \frac{|\Ical_{y}|}{n}.
$$
Moreover, for the second term on the right-hand side of \eqref{eq:8}, by using Lemma 1 of \citep{kawaguchi2022robust}, we have that with probability  at least $1-\delta$,
\begin{align*}
& \sum_{y\in \Ycal} \EE_{X_{y}}[\|W _{S}f_\theta(X_{y})-y \|]\left(\Pr(Y =  y)- \frac{|\Ical_{y}|}{n}\right) 
\\ &\le \left(\sum_{y\in \Ycal} \sqrt{p(y)}\EE_{X_{y}}[\|W _{S}f_\theta(X_{y})-y \| \right)   \sqrt{\frac{2\ln(|\Ycal|/\delta)}{2n}}
\\ & \le\kappa_{S} \left(\sum_{y\in \Ycal} \sqrt{p(y)} \right)   \sqrt{\frac{2\ln(|\Ycal|/\delta)}{2n}}
\end{align*} 
where $p(y)=\Pr(Y =  y)$.
Substituting this bound into \eqref{eq:8} with the union bound, we have that with probability at least $1-\delta$,
\begin{align} \label{eq:9} 
&\EE_{X,Y}[\|W _{S}f_\theta(X)-Y\|]   - \frac{1}{n} \sum_{i=1}^n \|W_{S}f_\theta(\bbx_i)-\bby_i\|
\\ \nonumber & \le \kappa_{S} \left(\sum_{y \in \tYcal} \sqrt{\hp(y)}\right)   \sqrt{\frac{\ln(2|\tYcal|/\delta)}{2n}} 
  +\kappa_{S} \left(\sum_{y\in \Ycal} \sqrt{p(y)} \right)   \sqrt{\frac{2\ln(2|\Ycal|/\delta)}{2n}}
  \\ \nonumber & \le \left(\sum_{y\in \Ycal} \sqrt{\hp(y)}\right)\kappa_{S}   \sqrt{\frac{2\ln(2|\Ycal|/\delta)}{2n}} 
  + \left(\sum_{y\in \Ycal} \sqrt{p(y)} \right) \kappa_{S}  \sqrt{\frac{2\ln(2|\Ycal|/\delta)}{2n}}   \\ \nonumber & \le\kappa_{S}   \sqrt{\frac{2\ln(2|\Ycal|/\delta)}{2n}}  \sum_{y\in \Ycal} \left(\sqrt{\hp(y)}+\sqrt{p(y)}\right) 
\end{align}
Combining \eqref{eq:1} and \eqref{eq:9} implies that with probability at least $1-\delta$,
\begin{align} \label{eq:10}
&\EE_{X,Y}[\|W _{S}f_\theta(X)-Y\|] 
\\ \nonumber  &\le  \frac{1}{n} \sum_{i=1}^n \|W_{S}f_\theta(\bbx_i)-\bby_i\|+\kappa_{S}   \sqrt{\frac{2\ln(2|\Ycal|/\delta)}{2n}}  \sum_{y\in \Ycal} \left(\sqrt{\hp(y)}+\sqrt{p(y)}\right)
  \\ \nonumber & \le L_{S}(w_{S})+\frac{1}{n} \sum_{i=1}^{n}\|\tW (f_\theta(\bbx_i)-f_\theta(x_i))\| 
\\ \nonumber & \quad + \frac{1}{n} \sum_{i=1}^n \|\varphi(x_{i})\|+\frac{1}{n} \sum_{i=1}^n\|\varphi(\bbx_i) \|+\kappa_{S}   \sqrt{\frac{2\ln(2|\Ycal|/\delta)}{2n}}  \sum_{y\in \Ycal} \left(\sqrt{\hp(y)}+\sqrt{p(y)}\right). 
\end{align}

We will now analyze  the term $\frac{1}{n} \sum_{i=1}^n \|\varphi(x_{i})\|+\frac{1}{n} \sum_{i=1}^n\|\varphi(\bbx_i) \|$ on the right-hand side of \eqref{eq:10}. Since $W^*=W_\bS$,
\begin{align*}
&\frac{1}{n} \sum_{i=1}^n \|\varphi(x_{i})\|=\frac{1}{n} \sum_{i=1}^n \|g^{*}(x_{i})-W_{\bS}f_\theta(x_{i})\|.
\end{align*}
By using Hoeffding's inequality (Lemma \ref{lemma:trivial:2}),  we have that for any $\delta>0$, with probability at least $1-\delta$, 
\begin{align*}
&\frac{1}{n} \sum_{i=1}^n \|\varphi(x_{i})\|\le \frac{1}{n} \sum_{i=1}^n \|g^{*}(x_{i})-W_{\bS}f_\theta(x_{i})\| \le \EE_{\xp}[\|g^{*}(\xp_{})-W_{\bS}f_\theta(\xp_{})\| ]+ \kappa_{\bS} \sqrt{\frac{\ln(1/\delta)}{2n} }.
\end{align*}
Moreover, by using  \citep[Theorem 3.1]{mohri2012foundations} with the  loss function $\xp \mapsto \|g^{*}(\xp_{})-Wf(\xp_{})\|$ (i.e., Lemma \ref{lemma:trivial:1}), we have that for any $\delta>0$, with probability at least $1-\delta$,
\begin{align} 
\EE_{\xp}[\|g^{*}(\xp_{})-W_{\bS}f_\theta(\xp_{})\| ]\le\frac{1}{m}\sum_{i=1}^{m} \|g^{*}(\xp_{i})-W_{\bS}f_\theta(\xp_{i})\|+\frac{2\tilde \Rcal_{m}(\Wcal \circ \Fcal)}{\sqrt{m}}+\kappa \sqrt{\frac{\ln(1/\delta)}{2m}} 
\end{align}
where $\tilde \Rcal_{m}(\Wcal \circ \Fcal)=\frac{1}{\sqrt{m}}\EE_{\bS,\xi}[\sup_{W\in \Wcal, f\in\Fcal} \sum_{i=1}^m \xi_i\|g^{*}(\xp_{i})-W_{}f(\xp_{i})\|]$ is the normalized Rademacher complexity of the set $\{\xp_{} \mapsto\|g^{*}(\xp_{})-W_{}f(\xp_{})\|:W \in \Wcal, f \in \Fcal\}$ (it is normalized such  that $\tilde \Rcal_{m}(\Fcal)=O(1)$  as $m\rightarrow \infty$
for typical choices of $\Fcal$), and $\xi_1,\dots,\xi_m$ are independent uniform random variables taking values in $\{-1,1\}$. Takinng union bounds, we have that for any $\delta>0$, with probability at least $1-\delta$, 
$$
\frac{1}{n} \sum_{i=1}^n \|\varphi(x_{i})\| \le\frac{1}{m}\sum_{i=1}^{m} \|g^{*}(\xp_{i})-W_{\bS}f_\theta(\xp_{i})\|+\frac{2\tilde \Rcal_{m}(\Wcal \circ \Fcal)}{\sqrt{m}}+\kappa \sqrt{\frac{\ln(2/\delta)}{2m}} + \kappa_{\bS} \sqrt{\frac{\ln(2/\delta)}{2n} }
$$ 
Similarly, for any $\delta>0$, with probability at least $1-\delta$, 
$$
\frac{1}{n} \sum_{i=1}^n \|\varphi(\bbx_{i})\| \le\frac{1}{m}\sum_{i=1}^{m} \|g^{*}(\xp_{i})-W_{\bS}f_\theta(\xp_{i})\|+\frac{2\tilde \Rcal_{m}(\Wcal \circ \Fcal)}{\sqrt{m}}+\kappa \sqrt{\frac{\ln(2/\delta)}{2m}} + \kappa_{\bS} \sqrt{\frac{\ln(2/\delta)}{2n}}.
$$
Thus, by taking union bounds, we have that for any $\delta>0$, with probability at least $1-\delta$,
\begin{align} \label{eq:18}
&\frac{1}{n} \sum_{i=1}^n \|\varphi(x_{i})\| +\frac{1}{n} \sum_{i=1}^n \|\varphi(\bbx_{i})\| \\ \nonumber & \le\frac{2}{m}\sum_{i=1}^{m} \|g^{*}(\xp_{i})-W_{\bS}f_\theta(\xp_{i})\|+\frac{4\Rcal_{m}(\Wcal \circ \Fcal)}{\sqrt{m}}+2\kappa \sqrt{\frac{\ln(4/\delta)}{2m}} + 2\kappa_{\bS} \sqrt{\frac{\ln(4/\delta)}{2n} }  
\end{align} 
To analyze the first term on the right-hand side of \eqref{eq:18},  recall that 
\begin{align} \label{eq:2}
W_{\bS} = \mini_{W'} \|W'\|_{F} \text{ s.t. } W'\in \argmin_{W} \frac{1}{m} \sum_{i=1}^{m} \|W f_\theta(\xp_{i})-g^*(\xp_i)\|^2 .
\end{align}
Here, since $W f_\theta(\xp_{i})\in\RR^r$, we have that 
$$
W f_\theta(\xp_{i}) = \vect[W f_\theta(\xp_{i})]=[f_\theta(\xp_{i})\T \otimes I_r]\vect[W]\in\RR^r,
$$ 
where $I_r \in \RR^{r \times r}
$ is the identity matrix, and $[f_\theta(\xp_{i})\T \otimes I_r]\in \RR^{r \times dr}$ is the  Kronecker product of the two matrices, and $\vect[W] \in \RR^{dr}$ is the vectorization of the matrix $W \in \RR^{r \times d}$.
Thus, by defining $A_i=[f_\theta(\xp_{i})\T \otimes I_r] \in \RR^{r \times dr}$  and using the notation of $w=\vect[W]$ and its inverse  $W=\vect^{-1}[w]$ (i.e., the inverse of the vectorization from $\RR^{r \times d}$ to $\RR^{dr}$ with a fixed ordering), we can rewrite \eqref{eq:2} by 
$$
W_\bS=\vect^{-1}[w_\bS] \quad \text{where } \quad w_\bS= \mini_{w'} \|w'\|_{F} \text{ s.t. } w'\in \argmin_{w} \sum_{i=1}^{m} \|g_{i}-A_iw\|^{2}, 
$$
with $g_i = g^{*}(\xp_{i}) \in \RR^r$. Since the function $w \mapsto \sum^{m}_{i=1} \|g_{i}-A_iw\|^{2}$ is convex, a necessary and sufficient condition of the minimizer of  this function is obtained by
$$
0 = \nabla_w \sum^{m}_{i=1} \|g_{i}-A_iw\|^{2}=2 \sum^{m}_{i=1} A_i\T (g_{i}-A_iw)\in \RR^{dr }
$$  
This implies that 
$$
\sum^{m}_{i=1}A_i\T A_iw= \sum^{m}_{i=1}A_i\T g_{i}.
$$
In other words, 
\begin{align*}
A\T A w=A\T g \quad \text{ where } A=\begin{bmatrix}A_{1} \\
A_{2} \\
\vdots \\
A_{m} \\
\end{bmatrix} \in \RR^{mr \times dr} \text{ and } g=\begin{bmatrix}g_{1} \\
g_{2} \\
\vdots \\
g_{m} \\
\end{bmatrix} \in \RR^{mr}
\end{align*}
Thus, 
$$
w'\in \argmin_{w} \sum_{i=1}^{m} \|g_{i}-A_iw\|^{2}= \{(A\T A)^\dagger A\T g+v: v \in \Null(A)\}
$$
where $(A\T A)^\dagger$ is the  Moore--Penrose inverse of the matrix  $A\T A$ and $\Null(A)$ is the null space of the matrix $A$. Thus, the minimum norm solution is obtained by 
$$
\vect[W_\bS]=w_\bS=(A\T A)^\dagger A\T g.
$$
Thus, by using this $W_\bS$, we have that 
\begin{align*}
\frac{1}{m}\sum_{i=1}^{m} \|g^{*}(\xp_{i})-W_{\bS}f_\theta(\xp_{i})\| &= \frac{1}{m}\sum_{i=1}^{m} \sqrt{\sum_{k=1}^r ((g_{i}-A_iw_\bS)_k)^2}
\\ & \le \sqrt{\frac{1}{m}\sum_{i=1}^{m} \sum_{k=1}^r ((g_{i}-A_iw_\bS)_k)^2} \\ & =  \frac{1}{\sqrt{m}} \sqrt{\sum_{i=1}^{m} \sum_{k=1}^r ((g_{i}-A_iw_\bS)_k)^2}
\\ & =\frac{1}{\sqrt{m}} \|g-Aw_\bS\|_{2}
\\ & = \frac{1}{\sqrt{m}} \|g-A(A\T A)^\dagger A\T g\|_{2} =\frac{1}{\sqrt{m}}\|(I-A(A\T A)^\dagger A\T )g\|_{2}
\end{align*}
where the inequality follows from the Jensen's inequality and the concavity of the square root function. 
Thus, we have that 
\begin{align} \label{eq:3}
&\frac{1}{n} \sum_{i=1}^n \|\varphi(x_{i})\| +\frac{1}{n} \sum_{i=1}^n \|\varphi(\bbx_{i})\| \\ \nonumber & \le\frac{2}{\sqrt{m}}\|(I-A(A\T A)^\dagger A\T )g\|_{2}+\frac{4\Rcal_{m}(\Wcal \circ \Fcal)}{\sqrt{m}}+2\kappa \sqrt{\frac{\ln(4/\delta)}{2m}} + 2\kappa_{\bS} \sqrt{\frac{\ln(4/\delta)}{2n} }  
\end{align}
By combining \eqref{eq:10} and  \eqref{eq:3} with union bound, we have that 
\begin{align} \label{eq:4}
&\EE_{X,Y}[\|W _{S}f_\theta(X)-Y\|] 
  \\ \nonumber & \le L_{S}(w_{S})+\frac{1}{n} \sum_{i=1}^{n}\|\tW (f_\theta(\bbx_i)-f_\theta(x_i))\|+\frac{2}{\sqrt{m}}\|\Pb_{A}g\|_{2} 
\\ \nonumber & \quad + \frac{4\Rcal_{m}(\Wcal \circ \Fcal)}{\sqrt{m}}+2\kappa \sqrt{\frac{\ln(8/\delta)}{2m}} + 2\kappa_{\bS} \sqrt{\frac{\ln(8/\delta)}{2n} }
\\ \nonumber  &\quad +\kappa_{S}   \sqrt{\frac{2\ln(4|\Ycal|/\delta)}{2n}}  \sum_{y\in \Ycal} \left(\sqrt{\hp(y)}+\sqrt{p(y)}\right). 
\end{align}
where $\tW=W_S-W^*$ and $   \Pb_{A}=I-A(A\T A)^\dagger A\T$.

We will now analyze the second term on the right-hand side of \eqref{eq:4}:
\begin{align} \label{eq:11}
\frac{1}{n} \sum_{i=1}^{n}\|\tW (f_\theta(\bbx_i)-f_\theta(x_i))\| \le \|\tW\|_{2}\ \left(\frac{1}{n} \sum_{i=1}^{n}\|f_\theta(\bbx_i)-f_\theta(x_i)\| \right),
\end{align} 
where $\|\tW\|_{2}$ is the spectral norm of $\tW$. Since $\bbx_i$ shares the same label with $x_i$ as  $\bbx_i \sim\Dcal_{y_i}$ (and $x_i \sim\Dcal_{y_i}$), and because $f_\theta$ is trained with the unlabeled data $\bS$,  using Hoeffding's inequality (Lemma \ref{lemma:trivial:2}) implies that with probability at least $1-\delta$, 
\begin{align} \label{eq:12}
\frac{1}{n} \sum_{i=1}^{n}\|f_\theta(\bbx_i)-f_\theta(x_i)\| \le \EE_{y \sim \rho}\EE_{\bbx,x \sim \Dcal_y^2}[\|f_\theta(\bbx)-f_\theta(x)\|]+\tau_{\bS} \sqrt{\frac{\ln(1/\delta)}{2n}}. 
\end{align}
Moreover, by using  \citep[Theorem 3.1]{mohri2012foundations} with the  loss function $(x,\bbx) \mapsto \|f_\theta(\bbx)-f_\theta(x)\|$ (i.e., Lemma \ref{lemma:trivial:1}), we have that with probability at least $1-\delta$,
\begin{align} 
\EE_{y \sim \rho}\EE_{\bbx,x \sim \Dcal_y^2}[\|f_\theta(\bbx)-f_\theta(x)\|] \le\frac{1}{m}\sum_{i=1}^{m} \|f_\theta(\xp_{i})-f_\theta(\xpp_{i})\|+\frac{2\tilde \Rcal_{m}(\Fcal)}{\sqrt{m}}+\tau \sqrt{\frac{\ln(1/\delta)}{2m}} 
\end{align}
where $\tilde \Rcal_{m}(\Fcal)=\frac{1}{\sqrt{m}}\EE_{\bS,\xi}[\sup_{f\in\Fcal} \sum_{i=1}^m \xi_i \|f(\xp_{i})-f(\xpp_{i})\|]$ is the normalized Rademacher complexity of the set $\{(\xp_{},\xpp_{}) \mapsto\|f(\xp_{})-f(\xpp_{})\|: f \in \Fcal\}$ (it is normalized such  that $\tilde \Rcal_{m}(\Fcal)=O(1)$  as $m\rightarrow \infty$
for typical choices of $\Fcal$), and $\xi_1,\dots,\xi_m$ are independent uniform random variables taking values in $\{-1,1\}$. Thus, taking union bound, we have that for any $\delta>0$, with probability at least $1-\delta$,
\begin{align} \label{eq:13}
&\frac{1}{n} \sum_{i=1}^{n}\|\tW (f_\theta(\bbx_i)-f_\theta(x_i))\|
\\ \nonumber & \le\|\tW\|_{2}\left(\frac{1}{m}\sum_{i=1}^{m} \|f_\theta(\xp_{i})-f_\theta(\xpp_{i})\|+\frac{2\tilde \Rcal_{m}(\Fcal)}{\sqrt{m}}+\tau \sqrt{\frac{\ln(2/\delta)}{2m}}++\tau_{\bS} \sqrt{\frac{\ln(2/\delta)}{2n}}\right). 
\end{align}

By combining \eqref{eq:4} and \eqref{eq:13} using the union bound, we have that with probability at least $1-\delta$,
\begin{align} \label{eq:14}
&\EE_{X,Y}[\|W _{S}f_\theta(X)-Y\|]
\\ \nonumber &\le L_{S}(w_{S}) + \|\tW\|_{2} \left( \frac{1}{m}\sum_{i=1}^{m} \|f_\theta(\xp_{i})-f_\theta(\xpp_{i})\|+\frac{2\tilde \Rcal_{m}(\Fcal)}{\sqrt{m}}+\tau \sqrt{\frac{\ln(4/\delta)}{2m}}+\tau_{\bS} \sqrt{\frac{\ln(4/\delta)}{2n}} \right)
\\ \nonumber & \quad +\frac{2}{\sqrt{m}}\|\Pb_{A}g\|_{2}+ \frac{4\Rcal_{m}(\Wcal \circ \Fcal)}{\sqrt{m}}+2\kappa \sqrt{\frac{\ln(16/\delta)}{2m}} + 2\kappa_{\bS} \sqrt{\frac{\ln(16/\delta)}{2n} }
\\ \nonumber & \quad +\kappa_{S}   \sqrt{\frac{2\ln(8|\Ycal|/\delta)}{2n}}  \sum_{y\in \Ycal} \left(\sqrt{\hp(y)}+\sqrt{p(y)}\right)
 \\ \nonumber & =L_{S}(w_{S}) +\|\tW\|_{2} \left(\frac{1}{m}\sum_{i=1}^{m} \|f_\theta(\xp_{i})-f_\theta(\xpp_{i})\|\right)+\frac{2}{\sqrt{m}}\|\Pb_{A}g\|_{2}+Q_{m,n} 
\end{align}
where
\begin{align*}
Q_{m,n} &= \|\tW\|_{2} \left(\frac{2\tilde \Rcal_{m}(\Fcal)}{\sqrt{m}}+\tau \sqrt{\frac{\ln(3/\delta)}{2m}}+\tau_{\bS} \sqrt{\frac{\ln(3/\delta)}{2n}}\right)
\\ & \quad +\kappa_{S}   \sqrt{\frac{2\ln(6|\Ycal|/\delta)}{2n}}  \sum_{y\in \Ycal} \left(\sqrt{\hp(y)}+\sqrt{p(y)}\right)
  \\ & \quad + \frac{4\Rcal_{m}(\Wcal \circ \Fcal)}{\sqrt{m}}+2\kappa \sqrt{\frac{\ln(4/\delta)}{2m}} + 2\kappa_{\bS} \sqrt{\frac{\ln(4/\delta)}{2n} }.
\end{align*}
Define $\hZ =[f(\xp_1),\dots, f(\xp_{m})] \in \RR^{d\times m}$. Then, we have $A=[\hZ \T \otimes I_r]$. Thus, 
$$
\Pb_{A}=I-[\hZ \T \otimes I_r][\hZ \hZ \T \otimes I_r]^\dagger[\hZ \otimes I_r]=I-[\hZ \T (\hZ \hZ \T)^\dagger \hZ \otimes I_r]=[\Pb_\hZ  \otimes I_r] 
$$
where $\Pb_\hZ  = I_{m}-\hZ \T (\hZ \hZ \T)^\dagger \hZ  \in \RR^{m \times m}$. By defining $Y_\bS=[g^*(\xp_1),\dots, g^*(\xp_{m})]\T \in \RR^{m\times r}$, since $g=\vect[Y_\bS\T]$,
\begin{align} \label{eq:15}
\| \Pb_{A}g\|_{2} =\|[\Pb_\hZ  \otimes I_r]\vect[Y_\bS\T]\|_{2} =\|\vect[Y_\bS\T\Pb_\hZ ]\|_{2} =\|\Pb_\hZ Y_\bS\|_{F}    
\end{align}
On the other hand, recall that $W_{S}$ is the minimum norm solution as 
$$
W_S =\mini_{W'} \|W'\|_{F} \text{ s.t. } W' \in \argmin_{W} \frac{1}{n} \sum_{i=1}^n \|W f_\theta(x_i)-y_i\|^2.
$$
By solving this,  we have  
$$
W_S =Y\T \tZ  \T (\tZ \tZ\T )^\dagger ,     
$$
where $\tZ =[f(x_1),\dots, f(x_{n})] \in \RR^{d\times n}$ and $Y_{S}=[y_{1},\dots, y_{n}]\T \in \RR^{n\times r}$. Then,
\begin{align*}
L_{S}(w_{S})=\frac{1}{n} \sum_{i=1}^n \|W_{S} f_\theta(x_i)-y_i\| &= \frac{1}{n}\sum_{i=1}^{n} \sqrt{\sum_{k=1}^r ((W_{S} f_\theta(x_i)-y_i)_k)^2} 
\\ & \le \sqrt{\frac{1}{n}\sum_{i=1}^{n}\sum_{k=1}^r ((W_{S} f_\theta(x_i)-y_i)_k)^2} \\ & =  \frac{1}{\sqrt{n}}  \|W_{S} \tZ -Y\T\|_F
\\ & =\frac{1}{\sqrt{n}}  \|Y\T (\tZ  \T (\tZ \tZ\T )^\dagger \tZ -I)\|_F
\\ & =\frac{1}{\sqrt{n}}  \|(I-\tZ  \T (\tZ \tZ\T )^\dagger \tZ )Y\|_F 
\end{align*} 
Thus, 
\begin{align} \label{eq:17}
L_{S}(w_{S})=\frac{1}{\sqrt{n}}  \|\Pb_\tZ Y\|_F
\end{align}
where $\Pb_\tZ   = I-\tZ  \T (\tZ \tZ\T )^\dagger \tZ $.

By combining \eqref{eq:14}--\eqref{eq:17} and using $1\le \sqrt{2}$, we have that with probability at least $1-\delta$,
\begin{align} 
\EE_{X,Y}[\|W _{S}f_\theta(X)-Y\|] \le c I_{\bS}(f_\theta)+\frac{2}{\sqrt{m}}\|\Pb_\hZ Y_\bS\|_{F}+\frac{1}{\sqrt{n}}  \|\Pb_\tZ Y_{S}\|_F +Q_{m,n}, 
\end{align}
where
\begin{align*}
Q_{m,n} &=  c \left(\frac{2\tilde \Rcal_{m}(\Fcal)}{\sqrt{m}}+\tau \sqrt{\frac{\ln(3/\delta)}{2m}}+\tau_{\bS} \sqrt{\frac{\ln(3/\delta)}{2n}}\right)
\\ & \quad +\kappa_{S}   \sqrt{\frac{2\ln(6|\Ycal|/\delta)}{2n}}  \sum_{y\in \Ycal} \left(\sqrt{\hp(y)}+\sqrt{p(y)}\right)
 \\ & \quad + \frac{4\Rcal_{m}(\Wcal \circ \Fcal)}{\sqrt{m}}+2\kappa \sqrt{\frac{\ln(4/\delta)}{2m}} + 2\kappa_{\bS} \sqrt{\frac{\ln(4/\delta)}{2n} }. 
\end{align*}
\end{proof}

\clearpage

\section{Known  Lemmas} 
We use the following well-known theorems as lemmas in our proof. We put these below for completeness.
These are classical results and \textit{not} our results.
\begin{lemma} \label{lemma:trivial:2}
\emph{(Hoeffding's inequality)} Let $X_1, ..., X_n$ be independent random variables such that ${\displaystyle a_{}\leq X_{i}\leq b_{}}$ almost surely. Consider the average of these random variables,
${\displaystyle S_{n}=\frac{1}{n}(X_{1}+\cdots +X_{n}).}$
Then,  for all $t > 0$,
$$
\PP_S \left( \mathrm {E} \left[S_{n}\right]-S_{n} \ge (b-a) \sqrt{\frac{\ln(1/\delta)}{2n} }\right) \leq \delta,
$$
and
$$
\PP_S \left( S_{n} -\mathrm {E} \left[S_{n}\right]\ge (b-a) \sqrt{\frac{\ln(1/\delta)}{2n} }\right) \leq \delta.
$$
\end{lemma}
\begin{proof}
By using Hoeffding's inequality, we have that
for all $t>0$,
$$
\PP_S \left( \mathrm {E} \left[S_{n}\right]-S_{n} \ge t\right)\leq \exp \left(-{\frac {2nt^{2}}{(b-a)^{2}}}\right),
$$
and 
$$
\PP_S \left(S_{n} - \mathrm {E} \left[S_{n}\right]\ge t\right)\leq \exp \left(-{\frac {2nt^{2}}{(b-a)^{2}}}\right),
$$
Setting $\delta=\exp \left(-{\frac {2nt^{2}}{(b-a)^{2}}}\right)$ and solving for $t>0$, 
\begin{align*}
& 1/\delta=\exp \left({\frac {2nt^{2}}{(b-a)^{2}}}\right) 
\\ & \Longrightarrow
\ln(1/\delta)= {\frac {2nt^{2}}{(b-a)^{2}}}
\\ & \Longrightarrow
\frac{(b-a)^{2}\ln(1/\delta)}{2n}= t^2
\\ & \Longrightarrow t =(b-a) \sqrt{\frac{\ln(1/\delta)}{2n} }
\end{align*} 
\end{proof}
It has been shown that   generalization bounds can be obtained via Rademacher complexity  \citep{bartlett2002rademacher,mohri2012foundations,shalev2014understanding}. The following  is a trivial modification of  \citep[Theorem 3.1]{mohri2012foundations} for a one-sided bound on the nonnegative general loss functions:
\begin{lemma} \label{lemma:trivial:1}
Let $\mathcal{G}$  be a  set of functions with the codomain  $[0, M]$. Then, for any $\delta>0$, with probability at least $1-\delta$ over  an i.i.d. draw of $m$ samples  $S=(q_{i})_{i=1}^m$, the following holds for all  $ \psi \in \Gcal$:
\begin{align}
\EE_{q}[\psi(q)]
\le \frac{1}{m}\sum_{i=1}^{m} \psi(q_{i})+2\Rcal_{m}(\Gcal)+M \sqrt{\frac{\ln(1/\delta)}{2m}}, \end{align}
where $\Rcal_{m}(\Gcal):=\EE_{S,\xi}[\sup_{\psi \in \Gcal}\frac{1}{m} \sum_{i=1}^m \xi_i \psi(q_{i})]$ and $\xi_1,\dots,\xi_m$ are independent uniform random variables taking values in $\{-1,1\}$. 
\end{lemma}
\begin{proof}
 Let $S=(q_{i})_{i=1}^m$ and $S'=(q_{i}')_{i=1}^m$. Define 
\begin{align}
\varphi(S)= \sup_{\psi \in \Gcal} \EE_{x,y}[\psi(q)]-\frac{1}{m}\sum_{i=1}^{m}\psi(q_{i}).
\end{align} 
To apply McDiarmid's inequality to $\varphi(S)$, we compute an upper bound on $|\varphi(S)-\varphi(S')|$ where  $S$ and $S'$ be two test datasets differing by exactly one point of an arbitrary index $i_{0}$; i.e.,  $S_i= S'_i$ for all $i\neq i_{0}$ and $S_{i_{0}} \neq S'_{i_{0}}$. Then,
\begin{align}
\varphi(S')-\varphi(S) \le\sup_{\psi \in \Gcal}\frac{\psi(q_{i_0})-\psi(q'_{i_0})}{m} \le \frac{M}{m}.
\end{align}
Similarly, $\varphi(S)-\varphi(S')\le \frac{M}{m} $.  Thus, by McDiarmid's inequality, for any $\delta>0$, with probability at least $1-\delta$,
\begin{align}
\varphi(S) \le  \EE_{S}[\varphi(S)] + M \sqrt{\frac{\ln(1/\delta)}{2m}}.
\end{align}
Moreover, 
\begin{align}
&\EE_{S}[\varphi(S)] 
\\ &  = \EE_{S}\left[\sup_{\psi \in \Gcal} \EE_{S'}\left[\frac{1}{m}\sum_{i=1}^{m}\psi_{}(q_i')\right]-\frac{1}{m}\sum_{i=1}^{m}\psi(q_i)\right]   
 \\ &  \le\EE_{S,S'}\left[\sup_{\psi \in \Gcal} \frac{1}{m}\sum_{i=1}^m (\psi(q'_i)-\psi(q_i))\right] 
 \\ & \le \EE_{\xi, S, S'}\left[\sup_{\psi \in \Gcal} \frac{1}{m}\sum_{i=1}^m  \xi_i(\psi_{}(q'_{i})-\psi(q_i))\right]
 \\ &  \le2\EE_{\xi, S}\left[\sup_{\psi \in \Gcal} \frac{1}{m}\sum_{i=1}^m  \xi_i\psi(q_i)\right] =2\Rcal_{m}(\Gcal)  
\end{align}
where  the first line follows the definitions of each term, the second line uses Jensen's inequality and the convexity of  the 
supremum, and the third line follows that for each $\xi_i \in \{-1,+1\}$, the distribution of each term $\xi_i (\ell(f_{}(x'_i),y'_i)-\ell(f(x_i),y_i))$ is the  distribution of  $(\ell(f_{}(x'_i),y'_i)-\ell(f(x_i),y_i))$  since $S$ and $S'$ are drawn iid with the same distribution. The fourth line uses the subadditivity of supremum.  
\end{proof}

\clearpage

\section{SimCLR}
In contrastive learning, different augmented views of the same image are attracted (positive pairs), while different augmented views are repelled (negative pairs). MoCo \citep{he2020momentum} and SimCLR \citep{chen2020simple} are recent examples of self-supervised visual representation learning that reduce the gap between self-supervised and fully-supervised learning. 
SimCLR applies randomized augmentations to an image to create two different views, $x$ and $y$, and encodes both of them with a shared encoder, producing representations $r_x$ and $r_y$. Both $r_x$ and $r_y$ are $l2$-normalized. The SimCLR version of the InfoNCE objective is:
\begin{align*}
    \mathbb{E}_{x,y}\left[-\log \left(\frac{e^{\frac1\eta r_y^Tr_x  }}{\sum_{k=1}^K{e^{\frac 1\eta r_{y_k}^Tr_x}}}\right)\right] ,
\end{align*}
where $\eta$ is a temperature term and $K$ is the number of views in a minibatch.

\section{Entropy Estimators }
Entropy estimation is one of the classical problems in information theory, where Gaussian mixture density is one of the most popular representations. With a sufficient number of components, they can approximate any smooth function with arbitrary accuracy. For Gaussian mixtures, there is, however, no closed-form solution to differential entropy. There exist several approximations in the literature, including loose upper and lower bounds \citep{entropyapprox2008}. Monte Carlo (MC) sampling is one way to approximate Gaussian mixture entropy. With sufficient MC samples, an unbiased estimate of entropy with an arbitrarily accurate can be obtained. Unfortunately, MC sampling is a very computationally expensive and typically requires a large number of samples, especially in high dimensions \citep{brewer2017computing}. Using the first two moments of the empirical distribution, VIGCreg used one of the most straightforward approaches for approximating the entropy. Despite this, previous studies have found that this method is a poor approximation of the entropy in many cases \cite{entropyapprox2008}. Another options is to use the LogDet function. Several estimators have been proposed to implement it, including uniformly minimum variance unbiased (UMVU) \citep{30996}, and bayesian methods \cite{MISRA2005324}. These methods, however, often require complex optimizations. The LogDet estimator presented in \cite{zhouyin2021understanding} used the differential entropy $\alpha$ order entropy using scaled noise. They demonstrated that it can be applied to high-dimensional features and is robust to random noise. Based on Taylor-series expansions, \cite{entropyapprox2008} presented a lower bound for the entropy of Gaussian mixture random vectors. They use Taylor-series expansions of the logarithm of each Gaussian mixture component to get an analytical evaluation of the entropy measure. In addition, they present a technique for splitting Gaussian densities to avoid components with high variance, which would require computationally expensive calculations. \cite{kolchinsky2017estimating} introduce a novel family of estimators for the mixture entropy. For this family, a pairwise-distance function between component densities defined for each member. These estimators are computationally efficient, as long as the pairwise-distance function and the entropy of each component distribution are easy to compute. Moreover, the estimator is continuous and smooth and is therefore useful for optimization problems. In addition, they presented both lower bound (using Chernoff distance) and an upper bound (using the KL divergence) on the entropy, which are are exact when the component distributions are grouped into well-separated clusters,
\label{app:methods}

% \section{Empirical validation of our assumption}
% \label{app:empiricalvalidation}
% We will try to verify empirically our assumptions on different datasets We compute the pairwise $l2$ distances between images for seven datasets: MNIST, CIFAR10, CIFAR100, Flowers102, Food101, and FGVAircaft.  We found that even for raw pixels, the pairwise distances are far from zero, which means you can use a small Gaussian around each point without overlapping. Consequently, the effective supports of these high-dimensional datasets are not overlapping, and our assumption is realistic even for current popular SSL datasets.

% \begin{figure}
%     \centering
%     \label{fig:overlapping}

%     \includegraphics[width=\linewidth]{figures/overlapping_proba.pdf}
%     \caption{\textbf{The Gaussians around each point are not overlapping} The $l2$ distances between raw images for different datasets}
%     \label{fig:my_label}
% \end{figure}

\section{EM, Information and collapsing}
\label{app:em}

Let us examine a toy dataset on the pattern of two intertwining moons to illustrate the collapse phenomenon under GMM (\Cref{fig:gaussian} - right). We begin by training a classical GMM with maximum likelihood, where the means are initialized based on random samples, and the covariance is used as the identity matrix. A red dot represents the Gaussian's mean after training, while a blue dot represents the data points. In the presence of fixed input samples, we observe that there is no collapsing and that the entropy of the centers is high (\Cref{fig:oneone} - left, in the Appendix). However, when we make the input samples trainable and optimize their location, all the points collapse into a single point, resulting in a sharp decrease in entropy (\Cref{fig:oneone} - right, in the Appendix).

To prevent collapse, we follow the K-means algorithm in enforcing sparse posteriors, i.e. using small initial standard deviations and learning only the mean. This forces a one-to-one mapping which leads all points to be closest to the mean without collapsing, resulting in high entropy (\Cref{fig:oneone} - middle, in the Appendix). Another option to prevent collapse is to use different learning rates for input and parameters. Using this setting, the collapsing of the parameters does not maximize the likelihood. \Cref{fig:gaussian} (right) shows the results of GMM with different learning rates for learned inputs and parameters. When the parameter learning rate is sufficiently high in comparison to the input learning rate, the entropy decreases much more slowly and no collapse occurs.

\section{Experimental Verification of Information-Based Bound Optimization}
\label{app:ver}

\textbf{Setup} Our experiments are conducted on CIFAR-10 \cite{krizhevsky2009learning}. We use ResNet-18 \citep{he2016deep} as our backbone. Each model is trained with $512$ batch size for $800$ epochs. We use linear evaluation to assess the quality of the representation. Once the model has been pre-trained, we follow the same fine-tuning procedures as for the baseline methods \citep{caron2020unsupervised}.

% \begin{table}[]
% \label{tab:results_app}
% \begin{tabular}{ll|l|}
% Method                       &                        & Accuracy                     \\ \hline 

% SimCLR                       &                       & $89.72 \pm 0.05$      \\
% \multicolumn{2}{l|}{Barlow Twins}                     & $88.81 \pm 0.1$        \\
% VICReg                       &                       & $89.32  \pm 0.09$      \\
% \multicolumn{2}{l|}{VICReg   + Pairwise Distances Estimator (ours)}     & $\mathbf{90.09 \pm 0.09}$       \\
% \multicolumn{2}{l|}{VICReg + Log Derminate Estimator (ours)} & $89.77  \pm 0.08$   \\ \hline 
% \end{tabular}

% \caption{\textbf{Entropy estimator achieved better results on SSL } - CIFAR10 accuracy on linear evaluation of SSL for different entropy estimators. The best results achieved by pairwise distances lower bound}

% \end{table}
% \section{Expectation Maximization and Collapsing}
\label{tab:em}
 \begin{figure}[t]
     \centering
     \includegraphics[width=\linewidth]{figures/GMM_entropies.png}
     \caption{Evolution of the entropy for each of the learning rate configurations showing that the impact of picking the incorrect learning rate for the data and/or centroids lead to a collapse of the samples.}
     \label{fig:entropies}
 \end{figure}

 \begin{figure}[t]
     \centering
     \includegraphics[width=\linewidth]{figures/GMM_one_one.pdf}
     \caption{\textbf{Evolution of GMM training when enforcing a one-to-one mapping between the data and centroids akin to K-means i.e. using a small and fixed covariance matrix. We see that collapse does not occur.} Left - In the presence of fixed input samples, we observe that there is no collapsing and
that the entropy of the centers is high. Right - when we make
the input samples trainable and optimize their location, all the points collapse into a single point,
resulting in a sharp decrease in entropy.}
     \label{fig:oneone}
 \end{figure}

\section{On Benefits of Information Maximization for Generalization} \label{app:1}
In this Appendix, we present the complete version of Theorem \ref{thm:1} along with its proof and additional discussions. 

\subsection{Additional Notation and details}

We start to introduce additional notation and details.  We use the notation of   $x \in \Xcal$ for an input and  $y \in \Ycal \subseteq \RR^r$ for an output. Define $p(y)=\Pr(Y=y)$ to be the probability of getting label $y$ and $\hp(y)=\frac{1}{n}\sum_{i=1}^n \one\{y_i=y\}$ to be the empirical estimate of $p(y)$.
Let $\zeta$  be an upper bound on the norm of the label as $\|y\|_{2} \le \zeta$ for all $y \in \Ycal$.
Define the  minimum norm solution $W_\bS$ of the unlabeled data as $W_\bS=\mini_{W'} \|W'\|_{F}$ s.t. $W'\in \argmin_W \frac{1}{m} \sum_{i=1}^{m} \|W_{} f_\theta(\xp_{i})-g^*(\xp_i)\|^2$. Let   $\kappa_{S}$  be a data-dependent upper bound on the per-sample Euclidian norm loss with the  trained model as $\|W_{S}f_\theta(x)-y\| \le \kappa_{S}$ for  all $(x,y) \in  \Xcal \times \Ycal$. Similarly, let $\kappa_{\bS}$  be a data-dependent upper bound on the per-sample Euclidian norm loss  as $\|W_{\bS}f_\theta(x)-y\| \le \kappa_{\bS}$ for  all $(x,y) \in  \Xcal \times \Ycal$. Define the difference between $W_S$ and $W_\bS$ by $c=\|W_S-W_\bS\|_{2}$. 
Let $\Wcal$ be a hypothesis space of $W$ such  that $W_\bS \in \Wcal$. We denote by  $\tilde \Rcal_{m}(\Wcal \circ \Fcal)=\frac{1}{\sqrt{m}}\EE_{\bS,\xi}[\sup_{W\in \Wcal, f\in\Fcal} \sum_{i=1}^m \xi_i\|g^{*}(\xp_{i})-W_{}f(\xp_{i})\|]$   the normalized Rademacher complexity of the set $\{\xp_{} \mapsto\|g^{*}(\xp_{})-W_{}f(\xp_{})\|:W \in \Wcal, f \in \Fcal\}$. we denote by $\kappa_{}$  a  upper bound on the per-sample Euclidian norm loss  as $\|Wf(x)-y\| \le \kappa_{}$ for  all $(x,y,W,f) \in  \Xcal \times \Ycal \times \Wcal\times \Fcal$.

We adopt the  following data-generating process model  that is used in  the previous paper  on analyzing contrastive learning \citep{saunshi2019theoretical, ben2018attentioned}. For the labeled data, first, $y$ is drawn  from the distritbuion $\rho$  on $\Ycal$, and then $x$ is drawn from the conditional distribution $\Dcal_{y}$ conditioned on the label $y$. That is, we have  the join distribution $\Dcal(x, y)=\Dcal _{y}(x)\rho(y)$ with $((x_i, y_i))_{i=1}^n \sim\Dcal^{n}$. For the unlabeled data,  first, each of the \textit{unknown} labels $y^{+}$ and $y^-$  is drawn  from the distritbuion $\rho$, and  then each of the  positive examples $\xp$ and $\xpp$ is drawn from the conditional distribution $\Dcal_{y^{+}}$ while the negative example  $\xn$ is  drawn from the  $\Dcal_{y^-}$.   Unlike the analysis of contrastive learning, we do not require the negative samples.
Let $\tau_{\bS}$  be a data-dependent upper bound on the invariance loss with the  trained representation as $\|f_\theta(\bbx)-f_\theta(x)\| \le \tau_{\bS}$   for all $(\bbx,x) \sim \Dcal_{y}^2$ and $y \in \Ycal$.
 Let   $\tau$  be a data-independent upper bound on the invariance loss with the  trained representation  as$ \|f(\bbx)-f(x)\| \le \tau$ for all $(\bbx,x) \sim \Dcal_{y}^2$, $y \in \Ycal$, and $f \in \Fcal$.  For the simplicity, we assume that there exists a function $g^*$ such that $y=g^{*}(x)\in \RR^r$ for all $(x,y) \in \Xcal \times \Ycal$. Discarding this assumption   adds the average of label noises to the final result, which goes to zero as the sample sizes $n$ and $m$ increase, assuming that the mean of the label noise is zero.

\end{appendices}
